# Supplementary material for: Fast phase prediction of charged polymer blends by white-box machine learning surrogates
Source: arXiv:2509.07164 ancillary file (2025-09-10)
Supplement: Supplementary file 1 [file si.pdf]

# Supporting Information for “Fast phase prediction of charged polymer blends by white-box machine learning surrogates”

## S1 Details of Random Phase Approximation

In this section, we provide a detailed description of the Random Phase Approximation (RPA) framework employed to determine phase behavior in charged polymer blends from 13-dimensional system parameters. The phase stability is governed by the inverse structure factor matrix  $\mathbf{S}^{-1}(k)$  defined in Eq. (1), which consists of two key components: the form factor matrix  $\mathbf{G}(k)$  that encodes segment-segment correlations along with average compositions of each component and the interaction matrix  $\mathbf{U}(k)$  that describes pairwise interactions between species. The explicit form of  $\mathbf{G}(k)$  and its block submatrices  $\mathbf{\Gamma}(\mathbf{x}, k)$  are defined in the main text. Here, we supplement these definitions by the details of the number densities attached to the  $\mathbf{\Gamma}$  blocks and the construction of  $\mathbf{U}(k)$ .

The number densities  $n_A/V, n_B/V, n_+/V, n_-/V, n_S/V$  attached to the  $\mathbf{\Gamma}$  blocks and other diagonal entries are a fast element of the RPA calculations. From the three composition parameters  $(\phi_S, f_A, f_p)$  described in the main text, we can determine the total volume fraction of solvent, polymer and counterions, and excess salt.

$$\phi_p = (1 - \phi_s)f_p, \quad (\text{S1})$$

$$\phi_{\pm}^{\text{ex}} = (1 - \phi_s)(1 - f_p). \quad (\text{S2})$$

Excess salt is differentiated from the volume fraction of small ions that compensate the charge asymmetry of the polymer, denoted  $\phi_{\pm}^0$ . In the case of where there is an excess polycation charge, small anions compensate. The composition can be solved via the following linear system

$$\begin{pmatrix} N_{A,c} & -N_{B,c} & -1 \\ 1 & 1 & 1 \\ 1 & 0 & f_A \end{pmatrix} \begin{pmatrix} \phi_A \\ \phi_B \\ \phi_{\pm}^0 \end{pmatrix} = \begin{pmatrix} 0 \\ \phi_p \\ f_A \phi_p \end{pmatrix}. \quad (\text{S3})$$

For charge symmetric polymers,  $\phi_{\pm}^0 = 0$ . The total small anion ion fraction is then

$$\phi_- = \phi_{\pm}^0 + \phi_{\pm}^{\text{ex}}/2, \quad (\text{S4})$$

$$\phi_+ = \phi_{\pm}^{\text{ex}}/2. \quad (\text{S5})$$

A similar linear system to Equation (S3) can be constructed when cations are necessary to compensate for the charge. Then the number density of each polymer species is

$$\frac{n_A}{V} = \frac{N_A \phi_A}{b^3}, \quad \frac{n_B}{V} = \frac{N_B \phi_B}{b^3}, \quad \frac{n_+}{V} = \frac{\phi_+}{a_+^3}, \quad \frac{n_-}{V} = \frac{\phi_-}{a_-^3}, \quad \frac{n_S}{V} = \frac{\phi_S}{b^3}. \quad (\text{S6})$$

The interaction matrix  $\mathbf{U}(k)$  is built from the pairwise interactions between each species. Within the RPA framework, it is convenient to use a monomer-level description of each species to build

the interaction matrix. Each polymer has charged and uncharged components, which we treat separately in the interaction matrix, leading to a  $7 \times 7$  matrix (two for each polymer, small cation, small ion, and solvent).

$$\mathbf{U}(k) = \begin{pmatrix} U_{A_u,A_u}(k) & U_{A_u,A_c}(k) & U_{A_u,B_u}(k) & U_{A_u,B_c}(k) & U_{A_u,+}(k) & U_{A_u,-}(k) & U_{A_u,S}(k) \\ U_{A_c,A_u}(k) & U_{A_c,A_c}(k) & U_{A_c,B_u}(k) & U_{A_c,B_c}(k) & U_{A_c,+}(k) & U_{A_c,-}(k) & U_{A_c,S}(k) \\ U_{B_u,A_u}(k) & U_{B_u,A_c}(k) & U_{B_u,B_u}(k) & U_{B_u,B_c}(k) & U_{B_u,+}(k) & U_{B_u,-}(k) & U_{B_u,S}(k) \\ U_{B_c,A_u}(k) & U_{B_c,A_c}(k) & U_{B_c,B_u}(k) & U_{B_c,B_c}(k) & U_{B_c,+}(k) & U_{B_c,-}(k) & U_{B_c,S}(k) \\ U_{+,A_u}(k) & U_{+,A_c}(k) & U_{+,B_u}(k) & U_{+,B_c}(k) & U_{+,+}(k) & U_{+,-}(k) & U_{+,S}(k) \\ U_{-,A_u}(k) & U_{-,A_c}(k) & U_{-,B_u}(k) & U_{-,B_c}(k) & U_{-,+}(k) & U_{-,-}(k) & U_{-,S}(k) \\ U_{S,A_u}(k) & U_{S,A_c}(k) & U_{S,B_u}(k) & U_{S,B_c}(k) & U_{S,+}(k) & U_{S,-}(k) & U_{S,S}(k) \end{pmatrix}, \quad (\text{S7})$$

where the  $u$  and  $c$  subscripts denote “uncharged” and “charged” monomers. In this work, we only consider contact interactions and direct electrostatic interactions. Any individual entry in the matrix above has the form

$$U_{i,j}(k) = \zeta + \chi_{i,j} + \frac{4\pi l_B z_i z_j}{k^2}, \quad (\text{S8})$$

where  $\zeta$  is the Helfand compressibility parameter used to enforce incompressibility for the system [1, 2]. Having  $\zeta \rightarrow \infty$  enforces incompressibility; however, we construct the compositions to satisfy incompressibility so the phase behavior is weakly dependent on the value of  $\zeta$ . The Coulomb term includes signed monomer valencies,  $z_{A_c} = z_+ = 1$  and  $z_B = z_- = -1$ . From symmetry, there are a total of 21 unique off-diagonal  $\chi_{i,j}$  pairs. By construction, we assign self interactions to be zero,  $\chi_{i,i} = 0$ . For monomers that only differ by their charge, we assume that equivalent  $\chi$  parameters, (i.e.  $\chi_{A_u,A_c} = \chi_{B_u,B_c} = 0$ ). These two assumptions significantly reduce the space to a set of 10  $\chi_{ij}$  parameters. We further reduce the space by focusing on a subset of physically meaningful interactions: incompatibility between polymers  $\chi_{A,B}$ , solvent-polymer interactions  $\chi_{A,S}$  and  $\chi_{B,S}$ , and ion-polymer interactions through a Born-like potential. As outlined in [3], a dielectric contrast between two polymer species manifests as a short-range attraction between small ions and the high dielectric polymer. Restricting ourselves to  $\epsilon_A/\epsilon_B > 1$  gives both  $\chi_{A,+}$  and  $\chi_{A,-}$ , calculated through

$$\chi_{A,\pm} = \frac{-l_B}{2a_{\pm}} \left( \frac{\epsilon_A}{\epsilon_B} - 1 \right). \quad (\text{S9})$$

The RPA workflow constructs the inverse structure factor matrix from

$$\mathbf{S}^{-1}(k) = \mathbf{G}^{-1}(k) + \mathbf{U}(k), \quad (\text{S10})$$

and the determinant of this matrix determines the stability of the homogeneous phase, which we use to construct phase boundaries. In cases of symmetry between species or when the volume fraction of a component is zero,  $\mathbf{S}(k)$  will not be full rank and we remove the corresponding rows and columns from  $\mathbf{G}(k)$  and  $\mathbf{U}(k)$  before computing the structure factor.

## S2 Phase Prediction and Data Generation

### S2.1 Incorporation of the PPGP surrogate into the RPA workflow

When calculating the inverse structure factor  $\mathbf{S}^{-1}(k)$ , the primary task is computing the inverse form factor  $\mathbf{G}(k)$ . Since  $\mathbf{G}(k)$  is block diagonal, its inverse has the form

$$\mathbf{G}^{-1}(k) = \begin{pmatrix} \frac{V^2}{n_A^2} \mathbf{\Gamma}^{-1}(\mathbf{x}_A, k) & & & & \\ & \frac{V^2}{n_B^2} \mathbf{\Gamma}^{-1}(\mathbf{x}_B, k) & & & \\ & & \frac{V}{n_+} & & \\ & & & \frac{V}{n_-} & \\ & & & & \frac{V}{n_S} \end{pmatrix}, \quad (\text{S11})$$

where the  $2 \times 2$  blocks  $\mathbf{\Gamma}^{-1}(\mathbf{x}_A, k)$  and  $\mathbf{\Gamma}^{-1}(\mathbf{x}_B, k)$  are inexpensive to evaluate once their entries are available.

The complete process for incorporating the surrogate predictions into the RPA workflow is as follows. First, compute  $\mathbf{x}_A = (N_{A,c}, N_{A,u})$  and  $\mathbf{x}_B = (N_{B,c}, N_{B,u})$  from  $r, \alpha_A, \alpha_B$  using  $N_A = 100, N_B = rN_A, N_{A,c} = N_A \alpha_A$ , and  $N_{A,u} = N_A - N_{A,c}$  with  $N_{B,c}$  and  $N_{B,u}$  defined analogously. Next, the white-box PPGP surrogate takes  $\mathbf{x}_A$  and  $\mathbf{x}_B$  as inputs to obtain predictions  $\hat{\mathbf{y}}(\mathbf{x}_A)$  and  $\hat{\mathbf{y}}(\mathbf{x}_B)$ , which are then exponentiated element-wise to recover  $\hat{G}_{11}(\mathbf{x}_A, k), \hat{G}_{12}(\mathbf{x}_A, k), \hat{G}_{22}(\mathbf{x}_A, k), \hat{G}_{11}(\mathbf{x}_B, k), \hat{G}_{12}(\mathbf{x}_B, k)$  and  $\hat{G}_{22}(\mathbf{x}_B, k)$  for  $k = k_1, \dots, k_m$ . These predictions yield determinants  $|\hat{\mathbf{\Gamma}}(\mathbf{x}_A, k)| = \hat{G}_{11}(\mathbf{x}_A, k)\hat{G}_{22}(\mathbf{x}_A, k) - (\hat{G}_{12}(\mathbf{x}_A, k))^2$  and  $|\hat{\mathbf{\Gamma}}(\mathbf{x}_B, k)| = \hat{G}_{11}(\mathbf{x}_B, k)\hat{G}_{22}(\mathbf{x}_B, k) - (\hat{G}_{12}(\mathbf{x}_B, k))^2$  and the inverses  $\hat{\mathbf{\Gamma}}^{-1}(\mathbf{x}_A, k)$  and  $\hat{\mathbf{\Gamma}}^{-1}(\mathbf{x}_B, k)$ . Substituting into Equation (6) gives the predicted block-diagonal  $\hat{\mathbf{G}}^{-1}(k)$ . Finally, the inverse structure factor is obtained as  $|\hat{\mathbf{S}}^{-1}(k)| = |\hat{\mathbf{G}}^{-1}(k) + \mathbf{U}(k)|$  for  $k = k_1, \dots, k_m$ , and the phase is determined by identifying the first  $k^*$  such that  $|\mathbf{S}^{-1}(k^*)| < 0$ .

### S2.2 Parameter Estimation for the PPGP Surrogate

For any set of  $n$  inputs  $\{\mathbf{x}_1, \dots, \mathbf{x}_n\}$ , denote the  $n \times 3m$  output as  $\mathbf{y} = (\mathbf{y}_1, \dots, \mathbf{y}_{3m})$  where  $\mathbf{y}_j = (y_j(\mathbf{x}_1), \dots, y_j(\mathbf{x}_n))^T$  for  $j = 1, \dots, 3m$ . Let  $\boldsymbol{\mu} = (\mu_1, \dots, \mu_{3m})$ ,  $\boldsymbol{\sigma}^2 = (\sigma_1^2, \dots, \sigma_{3m}^2)$ , and  $\boldsymbol{\gamma} = (\gamma_1, \gamma_2)$ . The parameters are estimated by maximizing the likelihood function. The full log-likelihood function of the PPGP model [4] is

$$\log L(\boldsymbol{\mu}, \boldsymbol{\sigma}^2, \boldsymbol{\gamma}, \eta \mid \mathbf{y}) = \sum_{j=1}^{3m} \left( -\frac{n}{2} \log(2\pi\sigma_j^2) - \frac{1}{2} \log |\mathbf{R} + \eta \mathbf{I}_n| - \frac{1}{2\sigma_j^2} (\mathbf{y}_j - \mathbf{1}_n \mu_j)^T (\mathbf{R} + \eta \mathbf{I}_n)^{-1} (\mathbf{y}_j - \mathbf{1}_n \mu_j) \right), \quad (\text{S12})$$

where  $\mathbf{R}$  is the correlation matrix defined by the Matérn kernel with roughness  $5/2$ ,  $\eta$  is the nugget, and  $\mathbf{1}_n$  is an  $n$ -dimensional vector of ones. Taking derivatives of Equation (S12) with respect to  $\mu_j$

and  $\sigma_j^2$  for each  $j = 1, \dots, 3m$  gives

$$\frac{\partial}{\partial \mu_j} \log L(\boldsymbol{\mu}, \boldsymbol{\sigma}^2, \boldsymbol{\gamma}, \eta \mid \mathbf{y}) = \frac{1}{\sigma_j^2} (\mathbf{1}_n^T (\mathbf{R} + \eta \mathbf{I}_n)^{-1} (\mathbf{y}_j - \mathbf{1}_n \mu_j)), \quad (\text{S13})$$

$$\frac{\partial}{\partial \sigma_j^2} \log L(\boldsymbol{\mu}, \boldsymbol{\sigma}^2, \boldsymbol{\gamma}, \eta \mid \mathbf{y}) = -\frac{n}{2\sigma_j^2} + \frac{1}{2\sigma_j^4} (\mathbf{y}_j - \mathbf{1}_n \mu_j)^T (\mathbf{R} + \eta \mathbf{I}_n)^{-1} (\mathbf{y}_j - \mathbf{1}_n \mu_j). \quad (\text{S14})$$

Setting the derivatives (S13) and (S14) to zero yields the maximum likelihood estimators  $\hat{\mu}_j = (\mathbf{1}_n^T (\mathbf{R} + \eta \mathbf{I}_n)^{-1} \mathbf{1}_n)^{-1} \mathbf{1}_n^T (\mathbf{R} + \eta \mathbf{I}_n)^{-1} \mathbf{y}_j$  and  $\hat{\sigma}_j^2 = (\mathbf{y}_j - \mathbf{1}_n \hat{\mu}_j)^T (\mathbf{R} + \eta \mathbf{I}_n)^{-1} (\mathbf{y}_j - \mathbf{1}_n \hat{\mu}_j) / n$ . Substituting  $\hat{\boldsymbol{\mu}} = (\hat{\mu}_1, \dots, \hat{\mu}_{3m})$  and  $\hat{\boldsymbol{\sigma}}^2 = (\hat{\sigma}_1^2, \dots, \hat{\sigma}_{3m}^2)$  into Equation (S12), the profile log-likelihood for  $(\boldsymbol{\gamma}, \eta)$  is

$$\log L(\boldsymbol{\gamma}, \eta \mid \mathbf{y}, \hat{\boldsymbol{\mu}}, \hat{\boldsymbol{\sigma}}^2) = -\frac{3m}{2} \log |\mathbf{R} + \eta \mathbf{I}_n| - \frac{n}{2} \sum_{j=1}^{3m} \log(S_j^2) + \text{Constant},$$

where  $S_j^2 = n\hat{\sigma}_j^2$ . The parameters  $\boldsymbol{\gamma}$  and  $\eta$  are estimated by numerically maximizing this profile likelihood based on the limited-memory Broyden–Fletcher–Goldfarb–Shanno algorithm (L-BFGS) optimization [5].

### S2.3 Phase Correction

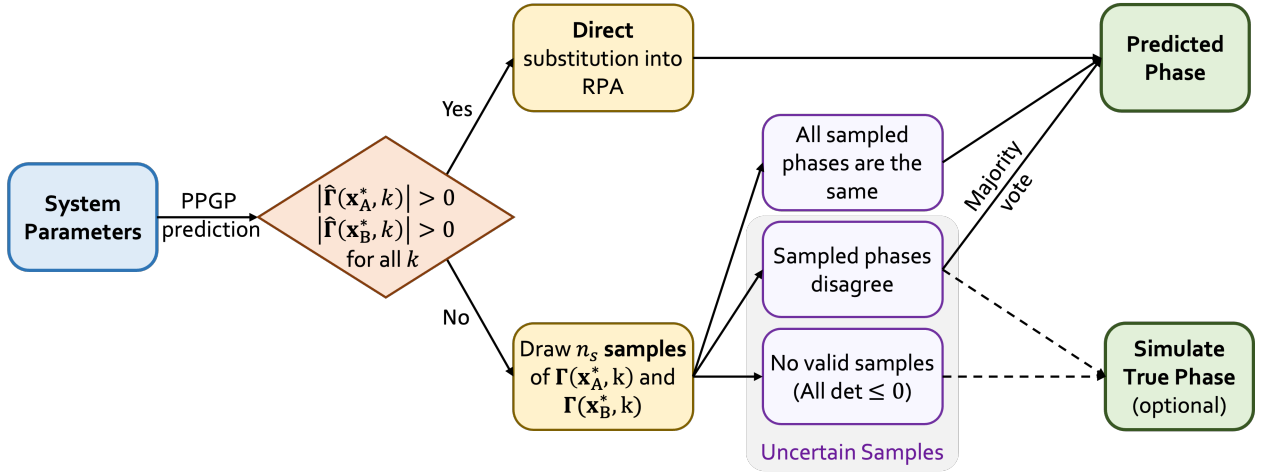

Figure S1: Flowchart of how a prediction is made using an initial input from the full parameter space. In the event that there is no majority agreement for the sampled phases or no physically valid samples, we cannot form a prediction and defer to the simulation if desired though this event is extremely rare for even small training dataset sizes.

Figure S1 illustrates how sampling is used to correct phase predictions that violate physical constraints ( $\Gamma(\mathbf{x}^*, k)$  must be positive definite for  $\mathbf{x}^* = \mathbf{x}_A^*$  or  $\mathbf{x}^* = \mathbf{x}_B^*$ ). When predicting  $\mathbf{y}(\mathbf{x}_A^*)$  and  $\mathbf{y}(\mathbf{x}_B^*)$  with the PPGP surrogate, if the resulting determinants of  $\Gamma(\mathbf{x}_A^*, k)$  and  $\Gamma(\mathbf{x}_B^*, k)$  are positive for all  $k = k_1, \dots, k_m$ , we directly substitute these predictions into the RPA calculation to obtain the predicted phase. If any predicted determinant is negative, we instead draw  $n_s$  samples from the predictive distribution (7). Only samples whose determinants are strictly positive for all  $k$

are retained and substituted into the RPA computation, which yields up to  $n_s$  sampled phases. The predicted phase is then determined by the majority vote among these sampled phases. For very small training size ( $n < 32$ ), there can be cases where none of the sampled outputs produce valid determinants (Figure 7). Together with predictions where multiple sampled phases arises (before applying the majority vote), one may directly resort to simulation to determine the true phase.

## S2.4 Data Generation

We generate the training inputs  $\mathbf{x}_1, \dots, \mathbf{x}_n$  using a sequential maximin design:

$$\mathbf{x}_{M+1} = \operatorname{argmax}_{\mathbf{x} \in \mathcal{X}} \min_{\mathbf{x}' \in X_0 \cup X_M} \|\mathbf{x} - \mathbf{x}'\|,$$

for  $M = n_0, \dots, n$ , where  $\|\cdot\|$  denotes the Euclidean norm,  $\mathcal{X} = \{(N_c, N_u) \mid 50 \leq N_c + N_u \leq 200, N_c, N_u \geq 1\}$  is the feasible region,  $X_0$  contains the discretized boundary of the region  $\mathcal{X}$  together with an initial batch  $\{\mathbf{x}_1, \dots, \mathbf{x}_{n_0}\}$  of  $n_0$  uniformly sampled training data points, and  $X_M = \{\mathbf{x}_1, \dots, \mathbf{x}_M\}$ . In practice, we use  $n_0 = 20$  initial uniformly sampled points. In contrast to a standard space-filling design such as maximin Latin hypercube sampling [6], this scheme biases the sampling toward the center of the feasible region. This is because boundary points are pre-included in  $X_0$ , so subsequent maximin selections preferentially fill the interior first, which is typically smoother and easier for the PPGP surrogate model to learn. As more points are added, regions closer to the boundary are gradually sampled, and the design eventually achieves space-filling of the entire domain.

## S3 Method Comparison

In addition to the proposed white-box PPGP model, we compare with three black-box classifiers: a neural network [7], random forest [8], and XGBoost [9, 10]. All of these models take the 13-dimensional system parameters as input and output the predicted phase among macrophase, microphase, and homogeneous.

The neural network is a composition of nonlinear functions

$$f(\mathbf{x}) = \sigma^{(L)}(\mathbf{W}^{(L)}\sigma^{(L-1)}(\dots\sigma^{(1)}(\mathbf{W}^{(1)}\mathbf{x} + \mathbf{b}^{(1)})\dots) + \mathbf{b}^{(L)}),$$

where  $\mathbf{W}^{(l)}$  are weight matrices of dimension  $d_l \times d_{l-1}$ ,  $\mathbf{b}^{(l)}$  are  $d_l$ -dimensional bias vectors, and  $\sigma^{(l)}$  are element-wise activation functions, for  $l = 1, \dots, L$ . We use  $L = 4$  with hidden layer widths  $d_1 = d_2 = d_3 = 512$ , input dimension  $d_0 = 13$ , and output dimension  $d_4 = 3$ . The hidden layers use ReLU activations  $\sigma^{(l)}(x_i) = \max(0, x_i)$ , and the output layer applies a softmax  $\sigma^{(L)}(x_i) = \exp(x_i) / \sum_{j=1}^{d_L} \exp(x_j)$  to produce phase probabilities. The predicted phase corresponds to the maximum probability.

Random forest is an ensemble tree method where each decision tree is trained on a bootstrap sample of the data and uses a random subset of features at each split. The ensemble prediction is obtained by majority vote across trees. We use the `randomForest` package [11] with 500 decision

trees and 3 randomly selected features per split which are the default settings in the package.

XGBoost is a boosting algorithm that builds decision trees sequentially, with each tree correcting the residual errors of the previous ensemble. Regularization is incorporated to reduce overfitting and improve efficiency. We use the `xgboost` package [10] with 100 boosting iterations, tree depth of 6, and learning rate of 0.3 corresponding to the default parameters in the package.

## S4 Additional Numerical Results

Here we present additional numerical results of our PPGP model. Figure S2 shows the NRMSE (Equation (10)) of the predictions for the entries  $G_{11}$ ,  $G_{12}$  and  $G_{22}$ , averaged over all  $k \in \{k_1, \dots, k_m\}$ , as training size increases from 20 to 250. The errors decrease rapidly as  $n$  grows, and all three entries plateau at  $n = 100$ . The cross-species term  $G_{12}$  consistently exhibits the largest error, due to greater difficulty in capturing cross-term correlations between charged and uncharged segments. Since the resulting phase prediction accuracy with  $n = 50$  already exceeds 99%, and improvements beyond this are negligible, we adopt  $n = 50$  training points in the final model.

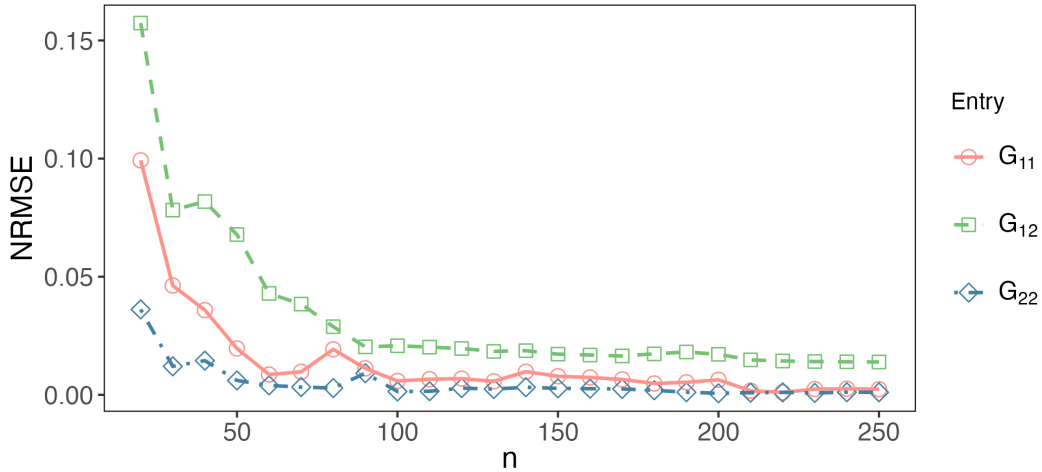

Figure S2: NRMSEs of surrogate predictions for  $G_{11}$ ,  $G_{12}$  and  $G_{22}$  as the training size increases from 20 to 250.

The uncertainty quantification of the PPGP model is evaluated using the length of the 95% credible interval for predictions, defined as

$$L_{g_1, g_2}(\mathbf{x}, k_j) = \hat{\sigma}_j \sqrt{K^*} (z_{0.975} - z_{0.025}), \quad (g_1, g_2) \in \{(1, 1), (1, 2), (2, 2)\}, \quad (\text{S15})$$

where  $\hat{\sigma}_j \sqrt{K^*}$  is the predictive standard deviation, with predictive variance defined in Equation (9), and  $z_{0.975}$  and  $z_{0.025}$  are the 97.5th and 2.5th quantiles of the standard normal distribution. Figure S3 shows the resulting interval lengths for predictions of  $G_{11}$ ,  $G_{12}$ ,  $G_{22}$  at  $k_1 = 10^{-2}$  from the surrogate model trained with  $n = 50$  points. Compared to the range of the true outputs (approximately  $[0, 10]$ ), these intervals are extremely narrow, indicating that the model is highly confident in its predictions.

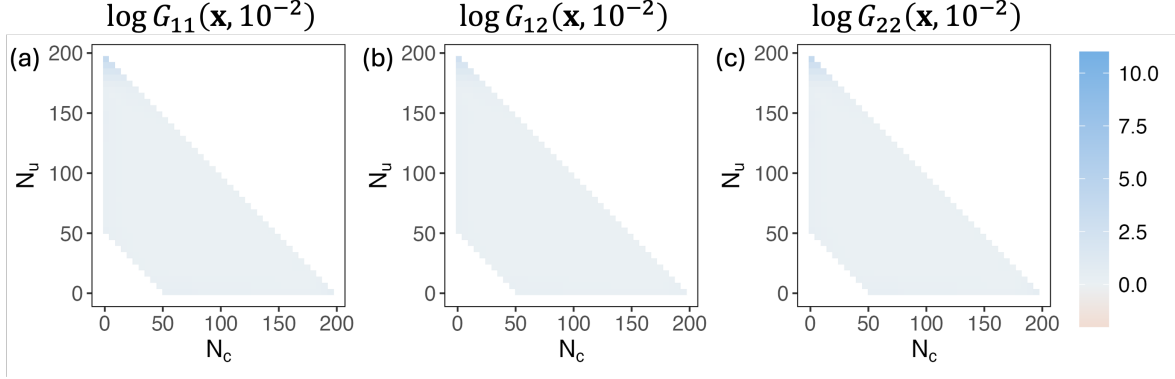

Figure S3: Lengths of 95% predictive intervals in Equation (S15) for predictions of  $\log G_{11}(\mathbf{x}, 10^{-2})$  (panel (a)),  $\log G_{12}(\mathbf{x}, 10^{-2})$  (panel (b)) and  $\log G_{22}(\mathbf{x}, 10^{-2})$  (panel (c)) from the surrogate model trained with  $n = 50$  points.

## References

- [1] Dominik Duchs, Kris T Delaney, and Glenn H Fredrickson. “A multi-species exchange model for fully fluctuating polymer field theory simulations”. In: *The Journal of Chemical Physics* 141.17 (2014).
- [2] Eugene Helfand. “Theory of inhomogeneous polymers: Fundamentals of the Gaussian random-walk model”. In: *Journal of Chemical Physics* 62.3 (1975), pp. 999–1005.
- [3] Douglas J Grzetic, Kris T Delaney, and Glenn H Fredrickson. “Electrostatic manipulation of phase behavior in immiscible charged polymer blends”. In: *Macromolecules* 54.6 (2021), pp. 2604–2616.
- [4] Mengyang Gu and James O Berger. “Parallel partial Gaussian process emulation for computer models with massive output”. In: *The Annals of Applied Statistics* 10.3 (2016), pp. 1317–1347.
- [5] Jorge Nocedal. “Updating quasi-Newton matrices with limited storage”. In: *Mathematics of computation* 35.151 (1980), pp. 773–782.
- [6] Thomas J Santner, Brian J Williams, and William I Notz. *The design and analysis of computer experiments*. Springer Science & Business Media, 2003.
- [7] Ian Goodfellow et al. *Deep learning*. Vol. 1. 2. MIT press Cambridge, 2016.
- [8] Leo Breiman. “Random forests”. In: *Machine learning* 45 (2001), pp. 5–32.
- [9] Jerome H Friedman. “Greedy function approximation: a gradient boosting machine”. In: *Annals of statistics* (2001), pp. 1189–1232.
- [10] Tianqi Chen and Carlos Guestrin. “XGBoost: A scalable tree boosting system”. In: *Proceedings of the 22nd acm sigkdd international conference on knowledge discovery and data mining*. 2016, pp. 785–794.
- [11] Andy Liaw and Matthew Wiener. “Classification and Regression by randomForest”. In: *R News* 2.3 (2002), pp. 18–22. URL: <https://CRAN.R-project.org/doc/Rnews/>.
